# Supplementary material for: Statistical mechanics of an elastically pinned membrane: Equilibrium dynamics and power spectrum
Source: arXiv:1806.10490 ancillary file (2018-06-27)
Supplement: Supplementary file 1 [file Supplementary_Information.pdf]

## Supplementary information

# Statistical mechanics of an elastically pinned membrane: Equilibrium dynamics and power spectrum

Josip A. Janeš,[1,2] Daniel Schmidt,[1,3] Udo Seifert,[3] and Ana-Sunčana Smith[1,2,*]

[1] *Institut für Theoretische Physik and Cluster of Excellence: Engineering of Advanced Materials, Friedrich Alexander Universität Erlangen-Nürnberg, 91052 Erlangen, Germany*
[2] *Institut Ruđer Bošković, 10000 Zagreb, Croatia*
[3] *II. Institut für Theoretische Physik, Universität Stuttgart, 70569 Stuttgart, Germany*

### CONTENTS

I. Power spectral density 1
  A. Spatio-temporal averaging of the power spectral density 2
    1. Spatial averaging over a circle of radius R 5

References 7

## I. POWER SPECTRAL DENSITY

Thermal equilibrium dynamics of a membrane profile $u(\mathbf{r},t)$ can be described by fluctuations $v(\mathbf{r},t)$ around the time-independent mean profile $\langle u(\mathbf{r})\rangle$ as

$$u(\mathbf{r},t) = \langle u(\mathbf{r})\rangle + v(\mathbf{r},t). \tag{1}$$

Power spectral density (PSD) of a membrane profile is defined as $\langle |v(\mathbf{r},\omega)|^2\rangle$, where $v(\mathbf{r},\omega)$ is the temporal Fourier transform of $v(\mathbf{r},t)$ and is given by (eq. (30) in the manuscript)

$$v(\mathbf{r},\omega) = \int_{\mathbb{R}^2} \mathrm{d}\mathbf{r}'\; g(\mathbf{r},\omega|\mathbf{r}')f(\mathbf{r}',\omega). \tag{2}$$

Here the frequency-space Green's function $g(\mathbf{r},\omega|\mathbf{r}')$ is given by (eq. (21) in the manuscript)

$$g(\mathbf{r},\omega|\mathbf{r}') = g_f(\mathbf{r}-\mathbf{r}',\omega) - \lambda \frac{g_f(\mathbf{r},\omega)g_f(\mathbf{r}',\omega)}{1+\lambda g_f(\mathbf{r}=0,\omega)}, \tag{3}$$

with the free-membrane Green's function

$$g_f(\tilde{\mathbf{r}},\omega) = \int_{\mathbb{R}^2} \frac{d\mathbf{k}}{(2\pi)^2} \frac{e^{i\mathbf{k}\tilde{\mathbf{r}}}}{i\omega/\Lambda_k + E_k} \tag{4}$$

and $f(\mathbf{r}',\omega)$ denotes the temporal Fourier transform of thermal forces characterized by

$$\langle f(\mathbf{r},\omega)f(\mathbf{r}',\omega')\rangle = 4\pi\Lambda^{-1}(\mathbf{r}-\mathbf{r}')\delta(\omega-\omega'). \tag{5}$$

Here $\Lambda^{-1}(\mathbf{r})$ is defined by

$$\Lambda(\mathbf{r}) * \Lambda^{-1}(\mathbf{r}) = \delta(\mathbf{r}) \tag{6}$$

and consequently

$$\mathcal{F}[\Lambda^{-1}(\mathbf{r})] = 1/\mathcal{F}[\Lambda(\mathbf{r})] \equiv \Lambda_k^{-1}, \tag{7}$$

* author to whom correspondence should be addressed: smith@physik.uni-erlangen.de

where $\mathcal{F}[\,]$ denotes the spatial Fourier transform, and

$$\int_{\mathbb{R}^2} \mathrm{d}\mathbf{r}_1' \int_{\mathbb{R}^2} \mathrm{d}\mathbf{r}_2' \; e^{-i\mathbf{k}_1\mathbf{r}_1'+i\mathbf{k}_2\mathbf{r}_2'} \Lambda^{-1}(\mathbf{r}_1'-\mathbf{r}_2') = (2\pi)^2 \delta(\mathbf{k}_1-\mathbf{k}_2)\Lambda_k^{-1}, \tag{8}$$

which will be used in the following calculation.

First step to calculating the PSD is finding $\langle v(\mathbf{r}_1,\omega_1)v^*(\mathbf{r}_2,\omega_2)\rangle$, which after inserting eqs. (2)-(8) becomes

$$\begin{aligned}
\langle v(\mathbf{r}_1,\omega_1)v^*(\mathbf{r}_2,\omega_2)\rangle &= \left\langle \left(\int_{\mathbb{R}^2} \mathrm{d}\mathbf{r}_1' g(\mathbf{r}_1,\omega_1|\mathbf{r}_1')f(\mathbf{r}_1',\omega_1)\right)\left(\int_{\mathbb{R}^2} \mathrm{d}\mathbf{r}_2' \; g(\mathbf{r}_2,\omega_2|\mathbf{r}_2')f(\mathbf{r}_2',\omega_2)\right)^* \right\rangle \\
&= \int_{\mathbb{R}^2} \mathrm{d}\mathbf{r}_1' \int_{\mathbb{R}^2} \mathrm{d}\mathbf{r}_2' \; g(\mathbf{r}_1,\omega_1|\mathbf{r}_1') \; g^*(\mathbf{r}_2,\omega_2|\mathbf{r}_2')\langle f(\mathbf{r}_1',\omega_1)f^*(\mathbf{r}_2',\omega_2)\rangle \\
&= 4\pi\delta(\omega_1-\omega_2)\times \int_{\mathbb{R}^2} \mathrm{d}\mathbf{r}_1' \int_{\mathbb{R}^2} \mathrm{d}\mathbf{r}_2' \; \left(g_f(\mathbf{r}_1-\mathbf{r}_1',\omega_1) - \frac{\lambda g_f(\mathbf{r}_1,\omega_1)g_f(\mathbf{r}_1',\omega_1)}{1+\lambda g_f(\mathbf{r}=0,\omega_1)}\right)\times \\
&\quad \times \left(g_f(\mathbf{r}_2-\mathbf{r}_2',\omega_2) - \frac{\lambda g_f(\mathbf{r}_2,\omega_2)g_f(\mathbf{r}_2',\omega_2)}{1+\lambda g_f(\mathbf{r}=0,\omega_2)}\right)^* \Lambda^{-1}(\mathbf{r}_1'-\mathbf{r}_2') \\
&= 4\pi\delta(\omega_1-\omega_2)\times \int_{\mathbb{R}^2} \mathrm{d}\mathbf{r}_1' \int_{\mathbb{R}^2} \mathrm{d}\mathbf{r}_2' \int_{\mathbb{R}^2} \frac{d\mathbf{k}_1}{(2\pi)^2} \frac{e^{i\mathbf{k}_1(\mathbf{r}_1-\mathbf{r}_1')}}{i\omega_1/\Lambda_{k_1}+E_{k_1}} \left(1-\frac{\lambda g_f(\mathbf{r}_1,\omega_1)}{1+\lambda g_f(\mathbf{r}=0,\omega_1)} e^{-i\mathbf{k}_1\mathbf{r}_1}\right)\times \\
&\quad \times \int_{\mathbb{R}^2} \frac{d\mathbf{k}_2}{(2\pi)^2} \frac{e^{-i\mathbf{k}_2(\mathbf{r}_2-\mathbf{r}_2')}}{-i\omega_2/\Lambda_{k_2}+E_{k_2}} \left(1-\frac{\lambda g_f(\mathbf{r}_2,\omega_2)}{1+\lambda g_f(\mathbf{r}=0,\omega_2)} e^{-i\mathbf{k}_2\mathbf{r}_2}\right)^* \Lambda^{-1}(\mathbf{r}_1'-\mathbf{r}_2') \\
&= 4\pi\delta(\omega_1-\omega_2)\times \int_{\mathbb{R}^2} \frac{d\mathbf{k}_1}{(2\pi)^2} \frac{e^{i\mathbf{k}_1\mathbf{r}_1}}{i\omega_1/\Lambda_{k_1}+E_{k_1}} \left(1-\frac{\lambda g_f(\mathbf{r}_1,\omega_1)}{1+\lambda g_f(\mathbf{r}=0,\omega_1)} e^{-i\mathbf{k}_1\mathbf{r}_1}\right)\times \\
&\quad \times \int_{\mathbb{R}^2} \frac{d\mathbf{k}_2}{(2\pi)^2} \frac{e^{-i\mathbf{k}_2\mathbf{r}_2}}{-i\omega_2/\Lambda_{k_2}+E_{k_2}} \left(1-\frac{\lambda g_f(\mathbf{r}_2,\omega_2)}{1+\lambda g_f(\mathbf{r}=0,\omega_2)} e^{-i\mathbf{k}_2\mathbf{r}_2}\right)^* \times \\
&\quad \times \int_{\mathbb{R}^2} \mathrm{d}\mathbf{r}_1' \int_{\mathbb{R}^2} \mathrm{d}\mathbf{r}_2' e^{-i\mathbf{k}_1\mathbf{r}_1'+i\mathbf{k}_2\mathbf{r}_2'} \Lambda^{-1}(\mathbf{r}_1'-\mathbf{r}_2') \\
&= 2\pi\delta(\omega_1-\omega_2)\times \frac{2}{(2\pi)^2}\int_{\mathbb{R}^2} \mathrm{d}\mathbf{k} \; e^{i\mathbf{k}(\mathbf{r}_1-\mathbf{r}_2)} \frac{\Lambda_k^{-1}}{(\omega_1/\Lambda_k)^2+E_k^2}\times \\
&\quad \times \left(1-\frac{\lambda g_f(\mathbf{r}_1,\omega_1)}{1+\lambda g_f(\mathbf{r}=0,\omega_1)} e^{-i\mathbf{k}\mathbf{r}_1}\right)\left(1-\frac{\lambda g_f(\mathbf{r}_2,\omega_1)}{1+\lambda g_f(\mathbf{r}=0,\omega_1)} e^{-i\mathbf{k}\mathbf{r}_2}\right)^*,
\end{aligned} \tag{9}$$

where eq. (8) was used in the last step. Setting $\mathbf{r}=\mathbf{r}_1=\mathbf{r}_2$ and $\omega=\omega_1=\omega_2$ in eq. (9) we find the power spectral density of a pinned membrane

$$\langle |v(\mathbf{r},\omega)|^2\rangle = \frac{2}{(2\pi)^2}\int_{\mathbb{R}^2} \mathrm{d}\mathbf{k} \frac{\Lambda_k^{-1}}{(\omega/\Lambda_k)^2+E_k^2} \left|1-\frac{\lambda g_f(\mathbf{r},\omega)}{1+\lambda g_f(\mathbf{r}=0,\omega)} e^{-i\mathbf{k}\mathbf{r}}\right|^2. \tag{10}$$

### A. Spatio-temporal averaging of the power spectral density

We start by showing that the Wiener-Khinchin theorem holds for averaged functions. For simplicity we show this for a one-dimensional function, as the reasoning for multidimensional functions is the same. We start with the one dimensional function of time $h(t)$ and its temporal average defined as

$$h_\tau(t) = \int_0^\tau \frac{\mathrm{d}t'}{\tau} h(t+t'). \tag{11}$$

We want to show that Wiener-Khinchin theorem holds for averaged functions, namely that the autocorrelation $C_\tau(t)$ of an averaged function is equal to the Fourier transform of an averaged power spectral density

$$C_\tau(t) \equiv \int_{-\infty}^{\infty} \mathrm{d}t' h_\tau^*(t') h_\tau(t+t') = \mathcal{F}\left[|h_\tau(\omega)|^2\right], \tag{12}$$

where $^*$ denotes complex conjugation and $h_T(\omega)$ is defined as a Fourier transform of $h_T(t)$:

$$\begin{aligned}
h_\tau(\omega) \equiv \mathcal{F}[h_\tau(t)] = &\int_{-\infty}^{\infty} dt\; e^{-i\omega t} \int_0^\tau \frac{\mathrm{d}t'}{\tau} h(t+t') \\
=&\int_0^\tau \frac{\mathrm{d}t'}{\tau} \int_{-\infty}^{\infty} dt\; e^{-i\omega t} h(t+t') \\
=&\int_0^\tau \frac{\mathrm{d}t'}{\tau} \int_{-\infty}^{\infty} dt''\; e^{-i\omega(t''-t')} h(t'') \\
=&\int_0^\tau \frac{\mathrm{d}t'}{\tau} e^{i\omega t'} \int_{-\infty}^{\infty} dt''\; e^{-i\omega t''} h(t'') \\
=&\int_0^\tau \frac{\mathrm{d}t'}{\tau} e^{i\omega t'} h(\omega) \\
=&e^{i\omega\tau/2} \frac{\sin(\omega\tau/2)}{\omega\tau/2} h(\omega).
\end{aligned} \tag{13}$$

We now show that eq. (12) holds.

$$\begin{aligned}
C_\tau(t) = &\int_{-\infty}^{\infty} \mathrm{d}t' h_\tau^*(t') h_\tau(t+t') \\
=&\int_{-\infty}^{\infty} \mathrm{d}t' \left( \int_0^\tau \frac{\mathrm{d}t_1'}{\tau} h^*(t'+t_1') \right) \left( \int_0^\tau \frac{\mathrm{d}t_2'}{\tau} h(t+t'+t_2') \right) \\
=&\int_{-\infty}^{\infty} \mathrm{d}t' \left( \int_0^\tau \frac{\mathrm{d}t_1'}{\tau} \left( \frac{1}{2\pi} \int_{-\infty}^{\infty} \mathrm{d}\omega h^*(\omega) e^{-i\omega(t'+t_1')} \right) \right) \left( \int_0^\tau \frac{\mathrm{d}t_2'}{\tau} \left( \frac{1}{2\pi} \int_{-\infty}^{\infty} \mathrm{d}\omega' h(\omega') e^{i\omega'(t+t'+t_2')} \right) \right) \\
=&\frac{1}{(2\pi)^2} \int_{-\infty}^{\infty} \mathrm{d}\omega \int_{-\infty}^{\infty} \mathrm{d}\omega' e^{i\omega' t} \left( \int_{-\infty}^{\infty} \mathrm{t}' e^{-it'(\omega-\omega')} \right) \left( \int_0^\tau \frac{\mathrm{d}t_1'}{\tau} e^{-i\omega t_1'} \right) \left( \int_0^\tau \frac{\mathrm{d}t_2'}{\tau} e^{i\omega' t_2'} \right) h^*(\omega) h(\omega') \\
=&\frac{1}{(2\pi)^2} \int_{-\infty}^{\infty} \mathrm{d}\omega \int_{-\infty}^{\infty} \mathrm{d}\omega' e^{i\omega' t} 2\pi\delta(\omega-\omega') \left( \int_0^\tau \frac{\mathrm{d}t_1'}{\tau} e^{-i\omega t_1'} \right) \left( \int_0^\tau \frac{\mathrm{d}t_2'}{\tau} e^{i\omega' t_2'} \right) h^*(\omega) h(\omega') \\
=&\frac{1}{2\pi} \int_{-\infty}^{\infty} \mathrm{d}\omega e^{i\omega t} \left( \int_0^\tau \frac{\mathrm{d}t_1'}{\tau} e^{-i\omega t_1'} \right) \left( \int_0^\tau \frac{\mathrm{d}t_2'}{\tau} e^{i\omega t_2'} \right) |h(\omega)|^2 \\
=&\frac{1}{2\pi} \int_{-\infty}^{\infty} \mathrm{d}\omega e^{i\omega t} \left| \left( \int_0^\tau \frac{\mathrm{d}t'}{\tau} e^{i\omega t'} \right) h(\omega) \right|^2 \\
\overset{(13)}{=}&\frac{1}{2\pi} \int_{-\infty}^{\infty} \mathrm{d}\omega e^{i\omega t} |h_\tau(\omega)|^2 \\
=&\mathcal{F}\left[ |h_\tau(\omega)|^2 \right]
\end{aligned} \tag{14}$$

Therefore, if we are interested in the autocorrelation of the averaged signal, we can first find its averaged spectrum and use the Wiener-Khinchin theorem (12), as with non-averaged signals.

We are interested in spatio-temporal signals averaged over time and space

$$u_\tau^A(\mathbf{r},t) = \int\limits_A \frac{\mathrm{d}\mathbf{r}}{A} \int\limits_0^\tau \frac{\mathrm{d}t'}{\tau} u(\mathbf{r}+\mathbf{r}', t+t'). \tag{15}$$

Using eq. (13), we find the averaged signal in the frequency domain

$$u_\tau^A(\mathbf{r},\omega) = e^{i\omega\tau/2}\frac{\sin(\omega\tau/2)}{\omega\tau/2} \int\limits_A \frac{\mathrm{d}\mathbf{r}'}{A} u(\mathbf{r}+\mathbf{r}',\omega). \tag{16}$$

Now calculating the averaged, mean-independent power spectral density

$$\begin{aligned}
\langle |v_\tau^A(\mathbf{r},\omega)|^2\rangle =& \langle v_\tau^A(\mathbf{r},\omega)\left(v_\tau^A(\mathbf{r},\omega)\right)^*\rangle \\
=& \left\langle \left(e^{i\omega\tau/2}\frac{\sin(\omega\tau/2)}{\omega\tau/2}\int\limits_A \frac{\mathrm{d}\mathbf{r}_1}{A} v(\mathbf{r}+\mathbf{r}_1,\omega)\right)\left(e^{i\omega\tau/2}\frac{\sin(\omega\tau/2)}{\omega\tau/2}\int\limits_A \frac{\mathrm{d}\mathbf{r}_2}{A} v(\mathbf{r}+\mathbf{r}_2,\omega)\right)^*\right\rangle \\
=& \left(\frac{\sin(\omega\tau/2)}{\omega\tau/2}\right)^2 \int\limits_A \frac{\mathrm{d}\mathbf{r}_1}{A}\int\limits_A \frac{\mathrm{d}\mathbf{r}_2}{A} \left\langle v(\mathbf{r}+\mathbf{r}_1,\omega)v^*(\mathbf{r}+\mathbf{r}_2,\omega)\right\rangle .
\end{aligned} \tag{17}$$

We have therefore reduced the task of temporal averaging just to a multiplication with a simple function in the frequency domain. We still have to do the spatial averaging. We use the result of eq. (9), valid for the case of a thermal stochastic force with zero mean, and insert it into eq. (17):

$$\begin{aligned}
\langle |v_\tau^A(\mathbf{r},\omega)|^2\rangle =& \left(\frac{\sin(\omega\tau/2)}{\omega\tau/2}\right)^2 \int\limits_A \frac{\mathrm{d}\mathbf{r}_1}{A}\int\limits_A \frac{\mathrm{d}\mathbf{r}_2}{A} \left\langle v(\mathbf{r}+\mathbf{r}_1,\omega)v^*(\mathbf{r}+\mathbf{r}_2,\omega)\right\rangle \\
=& \left(\frac{\sin(\omega\tau/2)}{\omega\tau/2}\right)^2 \int\limits_A \frac{\mathrm{d}\mathbf{r}_1}{A}\int\limits_A \frac{\mathrm{d}\mathbf{r}_2}{A} \frac{2}{(2\pi)^2}\int_{\mathbb{R}^2} \mathrm{d}\mathbf{k}\; e^{i\mathbf{k}(\mathbf{r}+\mathbf{r}_1-(\mathbf{r}+\mathbf{r}_2))}\frac{\Lambda_k^{-1}}{(\omega/\Lambda_k)^2+E_k^2} \\
& \left(1-\frac{\lambda g_f(\mathbf{r}+\mathbf{r}_1,\omega)}{1+\lambda g_f(\mathbf{r}=0,\omega)}e^{-i\mathbf{k}(\mathbf{r}+\mathbf{r}_1)}\right)\left(1-\frac{\lambda g_f(\mathbf{r}+\mathbf{r}_2,\omega)}{1+\lambda g_f(\mathbf{r}=0,\omega)}e^{-i\mathbf{k}(\mathbf{r}+\mathbf{r}_2)}\right)^* \\
=& \left(\frac{\sin(\omega\tau/2)}{\omega\tau/2}\right)^2 \frac{2}{(2\pi)^2}\int_{\mathbb{R}^2} \mathrm{d}\mathbf{k}\;\frac{\Lambda_k^{-1}}{(\omega/\Lambda_k)^2+E_k^2} \\
& \int\limits_A \frac{\mathrm{d}\mathbf{r}_1}{A} e^{i\mathbf{k}(\mathbf{r}+\mathbf{r}_1)}\left(1-\frac{\lambda g_f(\mathbf{r}+\mathbf{r}_1,\omega)}{1+\lambda g_f(\mathbf{r}=0,\omega)}e^{-i\mathbf{k}(\mathbf{r}+\mathbf{r}_1)}\right) \\
& \int\limits_A \frac{\mathrm{d}\mathbf{r}_2}{A} e^{-i\mathbf{k}(\mathbf{r}+\mathbf{r}_2)}\left(1-\frac{\lambda g_f(\mathbf{r}+\mathbf{r}_2,\omega)}{1+\lambda g_f(\mathbf{r}=0,\omega)}e^{-i\mathbf{k}(\mathbf{r}+\mathbf{r}_2)}\right)^* \\
=& \left(\frac{\sin(\omega\tau/2)}{\omega\tau/2}\right)^2 \frac{2}{(2\pi)^2}\int_{\mathbb{R}^2} \mathrm{d}\mathbf{k}\;\frac{\Lambda_k^{-1}}{(\omega/\Lambda_k)^2+E_k^2} \\
& \left|\int\limits_A \frac{\mathrm{d}\mathbf{r}'}{A} e^{i\mathbf{k}(\mathbf{r}+\mathbf{r}')}\left(1-\frac{\lambda g_f(\mathbf{r}+\mathbf{r}',\omega)}{1+\lambda g_f(\mathbf{r}=0,\omega)}e^{-i\mathbf{k}(\mathbf{r}+\mathbf{r}')}\right)\right|^2 \\
=& \left(\frac{\sin(\omega\tau/2)}{\omega\tau/2}\right)^2 \frac{2}{(2\pi)^2}\int_{\mathbb{R}^2} \mathrm{d}\mathbf{k}\;\frac{\Lambda_k^{-1}}{(\omega/\Lambda_k)^2+E_k^2} \\
& \left|\int\limits_A \frac{\mathrm{d}\mathbf{r}'}{A} e^{i\mathbf{k}(\mathbf{r}+\mathbf{r}')} - \frac{\lambda}{1+\lambda g_f(\mathbf{r}=0,\omega)}\int\limits_A \frac{\mathrm{d}\mathbf{r}'}{A} g_f(\mathbf{r}+\mathbf{r}',\omega)\right|^2 .
\end{aligned} \tag{18}$$

### *1. Spatial averaging over a circle of radius R*

For the PSD at $\mathbf{r}=0$, averaged over a circle with radius R, we find

$$\langle|v_\tau^A(\mathbf{r}=0,\omega)|^2\rangle = \left(\frac{\sin(\omega\tau/2)}{\omega\tau/2}\right)^2 \frac{2}{(2\pi)^2}\int_{\mathbb{R}^2} \mathrm{d}\mathbf{k}\ \frac{\Lambda_k^{-1}}{(\omega/\Lambda_k)^2+E_k^2}\left|\int\limits_A \frac{\mathrm{d}\mathbf{r}'}{A}e^{i\mathbf{k}\mathbf{r}'} - \frac{\lambda}{1+\lambda g_f(0,\omega)}\int\limits_A \frac{\mathrm{d}\mathbf{r}'}{A} g_f(\mathbf{r}',\omega)\right|^2$$

$$= \left(\frac{\sin(\omega\tau/2)}{\omega\tau/2}\right)^2 \frac{2}{(2\pi)^2}\int_{\mathbb{R}^2} \mathrm{d}\mathbf{k}\ \frac{\Lambda_k^{-1}}{(\omega/\Lambda_k)^2+E_k^2}\left|\frac{1}{R^2\pi}\int\limits_0^R \mathrm{d}r' r' \int\limits_0^{2\pi}\mathrm{d}\phi\ e^{i\mathbf{k}\mathbf{r}'} - \frac{\lambda}{1+\lambda g_f(0,\omega)}\frac{1}{R^2\pi}\int\limits_0^R \mathrm{d}r r\int\limits_0^{2\pi}\mathrm{d}\phi\ g_f(r',\omega)\right|^2$$

$$= \left(\frac{\sin(\omega\tau/2)}{\omega\tau/2}\right)^2 \frac{2}{(2\pi)^2}\int_{\mathbb{R}^2} \mathrm{d}\mathbf{k}\ \frac{\Lambda_k^{-1}}{(\omega/\Lambda_k)^2+E_k^2}\left|\frac{1}{R^2\pi}\int\limits_0^R \mathrm{d}r' r' 2\pi J_0(kr') - \frac{\lambda}{1+\lambda g_f(0,\omega)}\frac{1}{R^2\pi}\int\limits_0^R \mathrm{d}r' r' 2\pi g_f(r',\omega)\right|^2$$

$$= \left(\frac{\sin(\omega\tau/2)}{\omega\tau/2}\right)^2 \frac{2}{(2\pi)^2}\int_{\mathbb{R}^2} \mathrm{d}\mathbf{k}\ \frac{\Lambda_k^{-1}}{(\omega/\Lambda_k)^2+E_k^2}\frac{4}{R^4}\left|\int\limits_0^R \mathrm{d}r' r' J_0(kr') - \frac{\lambda}{1+\lambda g_f(0,\omega)}\int\limits_0^R \mathrm{d}r' r' \frac{1}{2\pi}\int\limits_0^\infty \mathrm{d}k' \frac{k' J_0(k'r')}{i\omega/\Lambda_{k'}+E_{k'}}\right|^2$$

$$= \left(\frac{\sin(\omega\tau/2)}{\omega\tau/2}\right)^2 \frac{2}{(2\pi)^2}\int_{\mathbb{R}^2} \mathrm{d}\mathbf{k}\ \frac{\Lambda_k^{-1}}{(\omega/\Lambda_k)^2+E_k^2}\frac{4}{R^4}\left|\frac{RJ_1(kR)}{k} - \frac{\lambda}{1+\lambda g_f(0,\omega)}\frac{1}{2\pi}\int\limits_0^\infty \mathrm{d}k' \frac{RJ_1(k'R)}{i\omega/\Lambda_{k'}+E_{k'}}\right|^2$$

$$= \left(\frac{\sin(\omega\tau/2)}{\omega\tau/2}\right)^2 \frac{2}{(2\pi)^2}\int_{\mathbb{R}^2} \mathrm{d}\mathbf{k}\ \frac{\Lambda_k^{-1}}{(\omega/\Lambda_k)^2+E_k^2}\frac{4}{R^2}\left|\frac{J_1(kR)}{k} - \frac{\lambda}{1+\lambda g_f(0,\omega)}\frac{1}{2\pi}\int\limits_0^\infty \mathrm{d}k' \frac{J_1(k'R)}{i\omega/\Lambda_{k'}+E_{k'}}\right|^2$$

$$= \left(\frac{\sin(\omega\tau/2)}{\omega\tau/2}\right)^2 \frac{1}{\pi}\int\limits_0^\infty \mathrm{d}k\ \frac{k\Lambda_k^{-1}}{(\omega/\Lambda_k)^2+E_k^2}\frac{4}{R^2}\left|\frac{J_1(kR)}{k} - \frac{\lambda}{1+\lambda g_f(0,\omega)}\frac{1}{2\pi}\int\limits_0^\infty \mathrm{d}k' \frac{J_1(k'R)}{i\omega/\Lambda_{k'}+E_{k'}}\right|^2. \tag{19}$$

For $\omega=0$, expression (19) becomes

$$\langle|v_\tau^A(\mathbf{r}=0,\omega=0)|^2\rangle = \frac{1}{\pi}\int\limits_0^\infty \mathrm{d}k\ \frac{k\Lambda_k^{-1}}{E_k^2}\frac{4}{R^2}\left|\frac{J_1(kR)}{k} - \frac{\lambda}{1+\lambda g_f(\mathbf{r}=0,\omega=0)}\frac{1}{2\pi}\int\limits_0^\infty \mathrm{d}k' \frac{J_1(k'R)}{E_{k'}}\right|^2. \tag{20}$$

We can get rid of the integral inside of the absolute value using [1]

$$g_f(\mathbf{r},\omega=0) = \frac{K_0(a_-|\mathbf{r}|)-K_0(a_+|\mathbf{r}|)}{2\pi\sqrt{\sigma^2-4\kappa\gamma}}, \tag{21}$$

with

$$a_\pm = \left[\frac{\sigma}{2\kappa}\left(1\pm\sqrt{1-\left(\frac{\lambda_m^0}{4\sigma}\right)^2}\right)\right]^{1/2}. \tag{22}$$

and

$$g_f(\mathbf{r}=0,\omega=0) = \frac{\arctan\left(\frac{\sqrt{4\kappa\gamma-\sigma^2}}{\sigma}\right)}{2\pi\sqrt{4\kappa\gamma-\sigma^2}} \equiv \frac{1}{\lambda_m}. \tag{23}$$

Starting with the frst row of eq. (19) and inserting $\omega = 0$ we find

$$\begin{aligned}\langle|v_\tau^A(\mathbf{r}=0,\omega=0)|^2\rangle =&\frac{2}{(2\pi)^2}\int_{\mathbb{R}^2}\mathrm{d}\mathbf{k}\,\frac{\Lambda_k^{-1}}{E_k^2}\left|\int\limits_A\frac{\mathrm{d}\mathbf{r}'}{A}e^{i\mathbf{k}\mathbf{r}'}-\frac{\lambda}{1+\lambda/\lambda_m}\int\limits_A\frac{\mathrm{d}\mathbf{r}'}{A}\,\frac{K_0(a_-|\mathbf{r}'|)-K_0(a_+|\mathbf{r}'|)}{2\pi\sqrt{\sigma^2-4\kappa\gamma}}\right|^2\\ =&\frac{2}{(2\pi)^2}\int_{\mathbb{R}^2}\mathrm{d}\mathbf{k}\,\frac{\Lambda_k^{-1}}{E_k^2}\left|\frac{J_1(kR)}{kR/2}-\frac{\lambda}{1+\lambda/\lambda_m}s(R)\right|^2\\ =&\frac{4\eta}{\pi}\int\limits_0^\infty\mathrm{dk}\,\frac{k^2}{E_k^2}\left|\frac{J_1(kR)}{kR/2}-\frac{\lambda}{1+\lambda/\lambda_m}s(R)\right|^2,\end{aligned}\tag{24}$$

where

$$s(R)=\frac{1}{R^2\pi\sqrt{\sigma-4\kappa\gamma}}\left(\frac{1-a_-RK_1(a_-R)}{a_-^2}-\frac{1-a_+RK_1(a_+R)}{a_+^2}\right).\tag{25}$$

We can invert expression (24) to find the value of the bond stiffness $\lambda$ from the measured PSD at the bond position. To that end we introduce the shorthand notation $L = \lambda/(1 + \lambda/\lambda_m) = \lambda\lambda_m/(\lambda + \lambda_m)$. With this notation eq. (20) becomes

$$\begin{aligned}\langle|v_\tau^A(\mathbf{r}=0,\omega=0)|^2\rangle =&\frac{4\eta}{\pi}\int\limits_0^\infty\mathrm{dk}\,\frac{k^2}{E_k^2}\left|\frac{J_1(kR)}{kR/2}-Ls(R)\right|^2\\ =&\frac{4\eta}{\pi}\int\limits_0^\infty\mathrm{dk}\,\frac{k^2}{E_k^2}\left(\left(\frac{J_1(kR)}{kR/2}\right)^2-2\frac{J_1(kR)}{kR/2}s(R)L+L^2s^2(R)\right).\end{aligned}\tag{26}$$

This is a quadratic equation for L:

$$aL^2-bL+c=0,\tag{27}$$

where the coefficients are given by

$$\begin{aligned}a=&\frac{\pi s^2(R)}{4\sqrt{\gamma(2\sqrt{\kappa\gamma}+\sigma)^3}},\\ b=&\frac{4s(R)}{R}\left(\int\limits_0^\infty\mathrm{dk}\frac{kJ_1(kR)}{E_k^2}\right),\\ c=&\left(\frac{2}{R}\right)^2\int\limits_0^\infty\mathrm{dk}\frac{J_1^2(kR)}{E_k^2}-\frac{\pi}{4\eta}\langle|v_\tau^A(\mathbf{r}=0,\omega=0)|^2\rangle.\end{aligned}\tag{28}$$

We see that the measured spectrum is contained in the coefficient $c$. By solving this quadratic equation for L with the choice of the "minus solution"

$$L=\frac{b}{2a}-\sqrt{\left(\frac{b}{2a}\right)^2-\frac{c}{a}}\tag{29}$$

and inserting this solution into

$$\lambda=\left(\frac{1}{L}-\frac{1}{\lambda_m}\right)^{-1}\tag{30}$$

we find the bond stiffness $\lambda$. This formula is not visually appealing, but is exact and its numerical calculation is practically instantaneous for an arbitrary big radius R. Therefore, if an experimental measure of the PSD of a membrane pinned with a single bond is available, this gives a valid and practical method for determining the value

of the bond stiffness $\lambda$ from the measured spectrum at the bond position. Of course, the spatial resolution of the measuring device, as well as the membrane parameters are assumed to be known.

[1] J. A. Janeš, H. Stumpf, S. D., S. U., and S. A.-S., ArXiv e-prints (2018), arXiv:1806.05109 [physics.bio-ph].
